# Supplementary material for: Deep Multitask Learning for Semantic Dependency Parsing
Source: arXiv:1704.06855 source file (2017-04-25)
Supplement: Supplementary file 1 [file supplementary.tex]

\section{Implementation Details}
\label{sec:implementation}
Each input token is mapped to a concatenation of three real vectors: a pre-trained word vector; a randomly-initialized word vector; and a randomly-initialized auxiliary POS tag vector.
All of them are tuned during training.
We use 100-dimensional \texttt{GloVe} \citep{pennington2014glove} trained over Wikipedia and Gigaword as pre-trained word embedding.
To deal with out-of-vocabulary words, we apply word dropout \citep{iyyer2015deep} and randomly replace a word $w$ with a special unk-symbol with probability $\frac{\alpha}{1 + \#(w)}$, where $\#(w)$ is the count of $w$ in the training set.

We make very limited attempts tuning the hyper-parameters.
The models are trained for up to 30 epochs with Adam \citep{kingma2014adam}, where $\beta_1, \beta_2 = 0.9$, and initial learning rate $\eta_0 = 1\times10^{-3}$. 
The learning rate $\eta$ is annealed at a rate of $0.5$ every 10 epochs \cite{dozat2016deep}.
We apply early-stopping based on the micro-averaged labeled ${F}_1$ score
on the development set.\footnote{Labeled ${F}_1$ score for the
single-task model.}
We set the maximum iteration number of $\mathrm{AD}^3$ to 500 and round the decisions when it doesn't converge.
$\ell_2$ norm of the gradient is clipped to 1 \citep{graves2013generating,sutskever2014sequence}, and we do not use mini-batches.
Randomly initialized parameters are sampled from a uniform distribution over $\bigl[-\sqrt{6/(d_{\mathrm{r}} + d_{\mathrm{c}})}, \sqrt{6/(d_{\mathrm{r}} + d_{\mathrm{c}})}\bigr]$, where $d_{\mathrm{r}}$ and $d_{\mathrm{c}}$ are the number of the rows and columns in the matrix, respectively. An $\ell_2$ penalty of $1\times10^{-6}$ is applied to all weights. Other hyper-parameters are summarized in Table \ref{tb:hyperparameters}. 

We use the same pruning technique as \citet{martins2014sdp}, where a first-order feature-rich unlabeled pruner is trained for each task, and arcs with posterior probability below $1\times10^{-4}$ are discarded. 
We further prune labeled structures which appear less than 30 times in the training set, and the label set sizes reduce to 39, 41, and 78 for DM, PAS, and PSD, respectively.
According to the statistics on the development set, about 10\% of the arcs remain after pruning, with a recall of around 99\%.

\begin{table}
\footnotesize
\begin{tabulary}{.48\textwidth}{c|C}
\Xhline{1pt}
  \textbf{Hyper-parameter} & \textbf{Value}\\
  \hline
  Pre-trained word embedding dimension & 100 \\
  Randomly-initialized word embedding dimension & 25 \\
  POS tag embedding dimension & 25 \\
  Dimensions of representations $\bm{\phi}$, $\widetilde{\bm{\phi}}$
  and $\bm{\psi}$ & 100\\
  BiLSTM layers & 2\\
  BiLSTM dimensions & 200 \\
  Rank of tensor $r$ & 100\\
  $\alpha$ for word dropout & 0.25\\
  \Xhline{1pt}
  
\end{tabulary}
\caption{Hyper-parameters used in the experiments.}
\label{tb:hyperparameters}
\end{table}
